# Supplementary material for: FlowIE: Efficient Image Enhancement via Rectified Flow
Source: arXiv:2406.00508 source file (2024-06-01)
Supplement: Supplementary file 2 [file derain1.tex]

\begin{figure*}[t]
    \centering
    \includegraphics[width=0.8\linewidth]{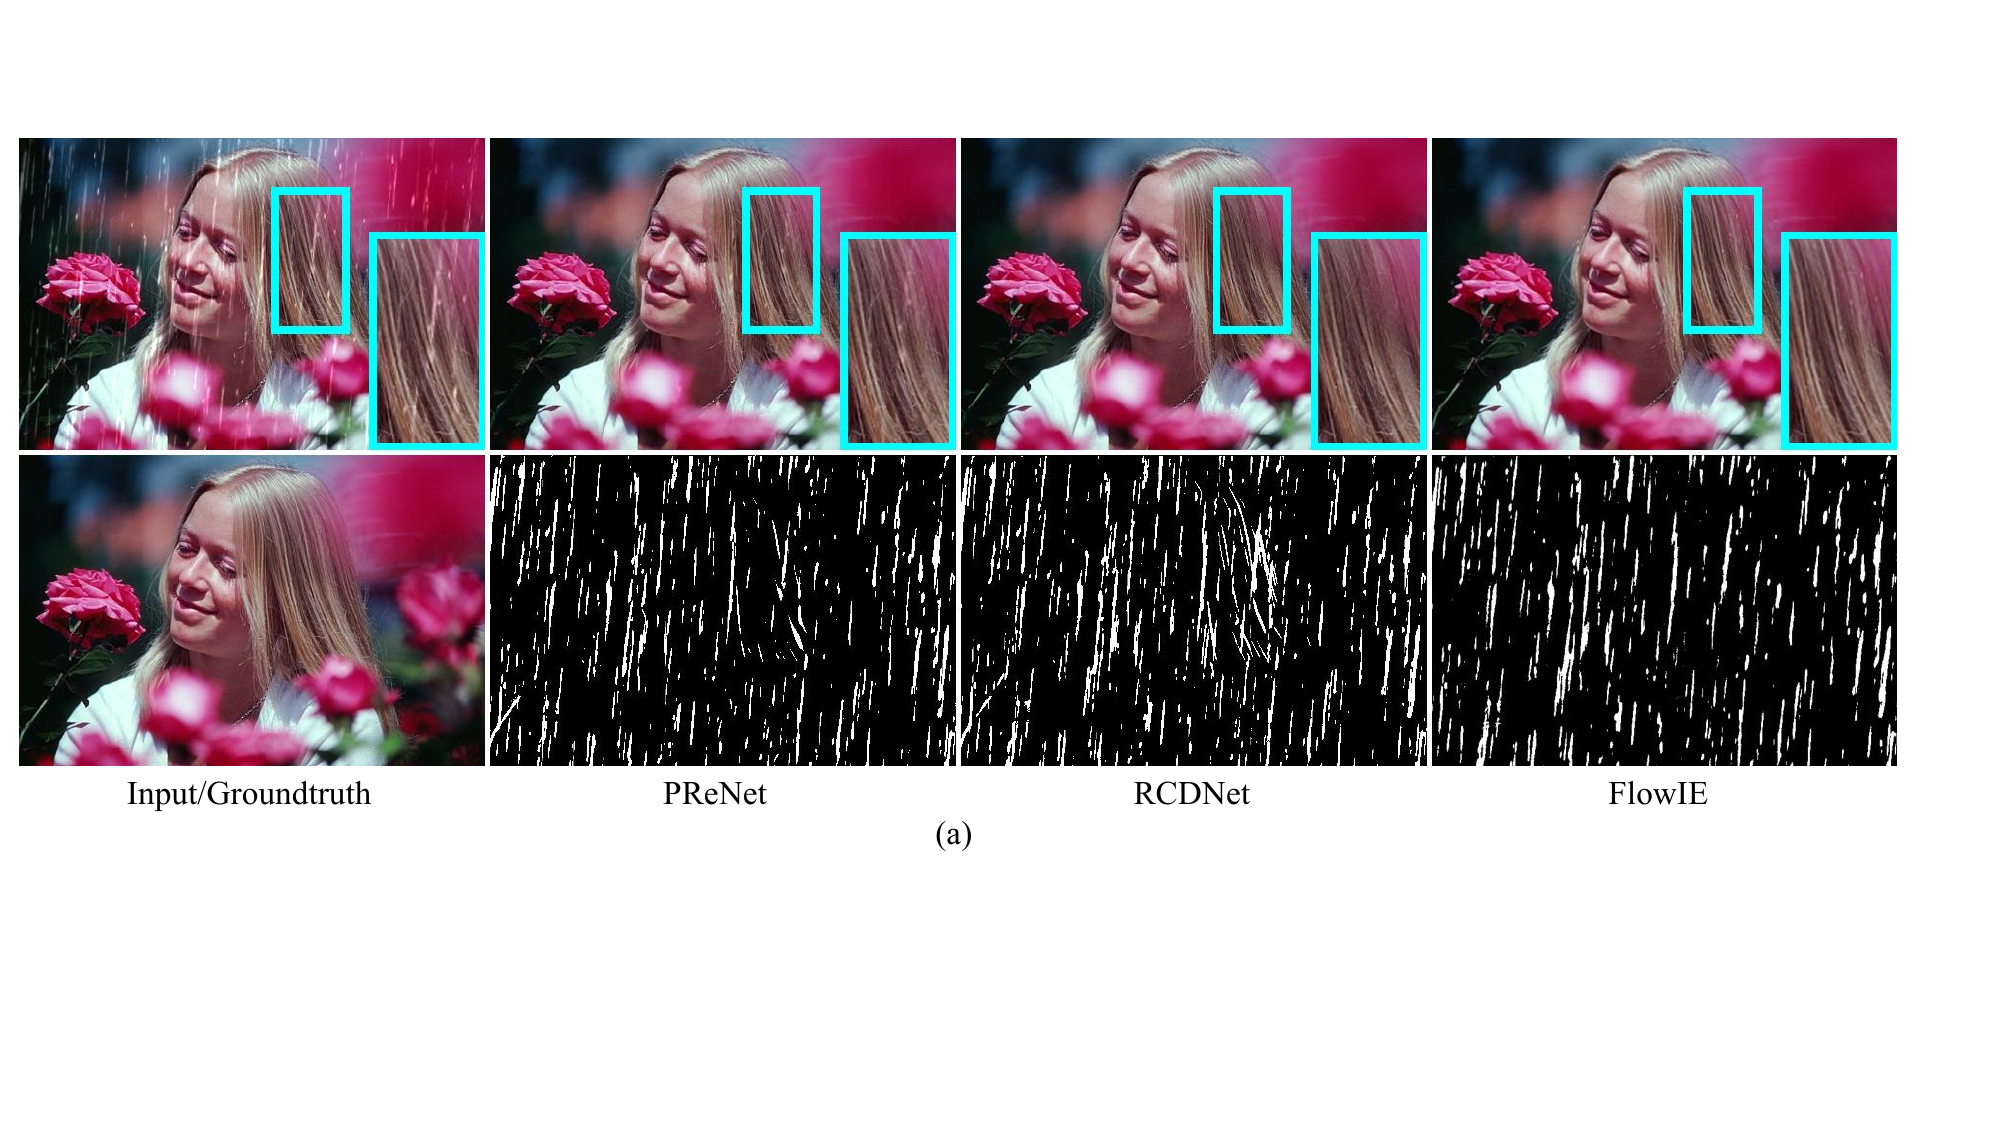}    
\end{figure*}
